# Supplementary material for: EvalResearchBench: Can AI Agents Build Their Own Feedback for Recursive Self-Improvement?
Source: arXiv:2610.04184 source file (2026-10-16)
Supplement: Supplementary file 1 [file appendix_case_study.tex]

\section{Final Artifact Case Study}
\label{app:sol-case}

We describe the final GPT-5.6 Sol/max artifact and its assessment contract. The researcher operated in a Python 3.12 sandbox with the supplied coding, co-work, and reasoning materials, a metered gateway, and fixed research and assessment wallets. The submitted program contains executable tasks, local and helper graders, frozen item weights, and three domain aggregations.

The final assessment retains completed wrong and empty responses as scores, marks infrastructure failures as missing, and records item-level completion, termination, and usage metadata. Domain scores are normalized weighted averages over completed items and enter the Score and PA comparisons under Section~\ref{sec:quality} on their submitted scale.

The artifact connects research inputs to executable tasks, graders, and independent measurements, with item-level coverage and cost records.
