# Supplementary material for: EvalResearchBench: Can AI Agents Build Their Own Feedback for Recursive Self-Improvement?
Source: arXiv:2610.04184 source file (2026-10-16)
Supplement: Supplementary file 2 [file appendix_design_analysis.tex]

\section{Researcher Artifact Notes}
\label{app:researcher-decisions}

The frozen artifacts differ in task composition, grading, and execution allowances.

\subsection{Astra and Sol}

The two frozen artifacts use different task compositions, graders, and execution allowances. Astra distributes weight across spreadsheet/data tasks, workflow rules, professional memos, and carried-context instructions; only the memo family uses helper grading. Sol uses structured coding, co-work, and reasoning suites with explicit per-request allowances. Both artifacts retain completed wrong and empty answers, exclude infrastructure failures, and expose item-level completion metadata.

The resulting measurements differ by domain. Astra's overall PA is 69.54\%, compared with Sol's 63.32\% (Table~\ref{tab:main-results}); their overall Score values are 22.79 and 16.99. The comparison links two concrete design profiles to their independently measured outcomes.

\subsection{K3 and Astra}
\label{app:k3-astra-decisions}

K3 and Astra both combine executable coding tasks, professional-work scenarios, and structured reasoning problems. Their final artifacts differ in task families and scoring rules. K3 reaches 74.58\% overall PA, compared with Astra's 69.54\% (Table~\ref{tab:main-results}). The representative target scatterplots in Figure~\ref{fig:family-scatter} show how score agreement and candidate ordering can differ.

The public comparison uses the independently assessed frozen artifact, with item coverage recorded alongside the results.
